# Supplementary material for: "Business on WhatsApp is tough now -- but am I really a businesswoman?" Exploring Challenges with Adapting to Changes in WhatsApp Business
Source: arXiv:2502.10913 source file (2025-02-15)
Supplement: Supplementary file 1 [file appendix.tex]

\appendix
\section{Appendix}
\label{appendix}
